# Supplementary material for: GANav: Efficient Terrain Segmentation for Robot Navigation in Unstructured Outdoor Environments
Source: arXiv:2103.04233 source file (2022-06-18)
Supplement: Supplementary file 1 [file bellsandwhistle.tex]

\section{Bells and Whistles}
\subsection{Dynamic Weighting}
\label{dw}
Models trained on datasets with long-tailed distribution of classes can be biased towards the most frequent classes. There are  many techniques~\cite{zhang2018generalized, cui2019classbalanced} to re-weight classes or effective samples to deal with label corruption and long-tailed distribution by giving priority to rare classes. To assist the model in learning feature representations for all classes uniformly, we adapt a weighted cross-entropy loss function in which the weights are determined by a new dynamic weighting strategy based on class error rate.% which is proven to be useful in Section~\ref{exp}. 

Let the weights at the first epoch be $W_{init} \in \mathbb{R}^G$ and the weights at the $i^{th}$ epoch be $W_{i} \in \mathbb{R}^G$. After $d$ more epochs, the weight update rule is given as: 

\begin{equation}
     \mathcal{W}_{i+d} = m * W_{i} + (1 - m) * (W_{init} + W^d_{error}),
     \label{eq: dw_equation}
\end{equation}
where $m$ is the momentum and $W^d_{error}\in[0, 1]^G$ is the error rate of each group during the intermediate $d$ epochs. 

The momentum term assures that the change in weights is not drastic. Thus, the dynamic weighting scheme increments the weights in small steps. Additionally, our method can adaptively assign weights in accordance with the training stage. The usage of the initial weights in the second term prevents bias towards a specific class. %using the initial weighting from the second term.% 
Our dynamic weighting scheme aims to make small adjustments based on the initial weighting from the hyper-parameters. 
% With dynamic weight, we achieve an improvement of 3.76\% in mean accuracy for RELLIS-3D dataset.
