# Supplementary material for: GANav: Efficient Terrain Segmentation for Robot Navigation in Unstructured Outdoor Environments
Source: arXiv:2103.04233 source file (2022-06-18)
Supplement: Supplementary file 2 [file group_analysis.tex]

\section{More Analysis on Effect of Grouping}
\label{error_more}
In this section, we include more comparison results on the effect of grouping in \ref{tab:error2}. In most of cases, grouping can improve the accuracy drastically, up to 61.65\% in some groups. It's inevitable that, for some groups, the performance degraded within a margin of 3.5\%. Overall, with grouping, we have a higher accuracy during training without losing the necessary information, as we distinguish all semantically different labels relevant to the task.

In addition, we show our method and some comparison methods with different grouping schemes in Table~\ref{tab:comparison_back}.
