# Supplementary material for: GANav: Efficient Terrain Segmentation for Robot Navigation in Unstructured Outdoor Environments
Source: arXiv:2103.04233 source file (2022-06-18)
Supplement: Supplementary file 3 [file implementation_details.tex]

\section{More Implementation Details}

We use \cite{mmseg2020} as our baseline and build on top of their code, which can be found at \url{https://github.com/open-mmlab/mmsegmentation}. 

% We integrate BoT~\cite{srinivas2021bottleneck} and our detection head in the framework, and use the methods in their implementation for comparisons.

\subsection{Architecture}
We implement the backbone architecture described in \cite{srinivas2021bottleneck}, which replaces the convolution layers with MHSA during the last stage of ResNet-50. 

Our detection head takes the output of the BoT backbone and first send the input to a MHSA layer with a hidden dimension of 2048. Then the output was propagated through a fully connected layer with the 2048 channels and reshaped to the same size as the original input. The output was concatenated with the original input for skip connection. Finally, we propagate the output through a 3x3 2d conv and another fully connected layer.

\subsection{Training details}

To obtain the pre-trained model, we first train the BoT backbone on the corresponding datasets with 80K iterations. Then we use another 80K iterations by loading the pre-trained model.
