# Supplementary material for: GANav: Efficient Terrain Segmentation for Robot Navigation in Unstructured Outdoor Environments
Source: arXiv:2103.04233 source file (2022-06-18)
Supplement: Supplementary file 4 [file realworld.tex]

\section{More Navigation Details and Results }

In this section, we add more details about our real-world implementation and navigation results. We show an image of our Jackal and Husky robot in Fig.~\ref{fig:robot}.

% \input{Tables/route}

% In table~\ref{tab:route}, we include details about each route.
In table~\ref{tab:breakdown}, we breakdown the navigation results for each scenario. The only case in which our method failed is when \ours{} misclassified a brick road as obstacles. We show some more qualitative results in Fig.~\ref{fig:realworld}.
