# Supplementary material for: GANav: Efficient Terrain Segmentation for Robot Navigation in Unstructured Outdoor Environments
Source: arXiv:2103.04233 source file (2022-06-18)
Supplement: Supplementary file 5 [file visual_results.tex]

\section{More Visualizations in Different Scenarios}

We include more visual results from our methods on RUGD in Fig.~\ref{fig:visualisations2} and RELLIS-3D in Fig.~\ref{fig:visualisations3}.
\vspace{10mm}
% \newpage
% \clearpage
